# Supplementary material for: Are Graph Neural Networks Optimal Approximation Algorithms?
Source: arXiv:2310.00526 source file (2024-10-04)
Supplement: Supplementary file 1 [file additional.tex]

Most algorithms can be organized into surprisingly few paradigms such as dynamic programming, convex optimization, divide and conquer, etc.  This observation becomes especially striking when dealing with fundamental NP-hard problems.  It is known, that for a remarkably broad class of problems--max cut, vertex cover, graph coloring, and any max constraint satisfaction problem--improving on the best approximation algorithms would be impossible if the so called unique games conjecture is true.  Perhaps equally remarkably, there is a class of algorithms that is known to be optimal amongst the polynomial time algorithms for max constraint satisfaction problems and it is given by a specific SDP relaxation.  Of course, this algorithm is only "efficient" theoretically, % in quotes, 
and does not preclude better approximation algorithms that could adapt to the data distribution over instances.  In this sense, it is critical that an optimal approximation comes from a learning algorithm that in the worst case still matches the performance of a powerful convex relaxation.  This is the driving question of our work.

\textit{"Is there an approximation algorithm that can learn to adapt to a data distribution over instances yet retain the optimal worst case performance of convex relaxations?"}
\[
\pE_\mu[\textbf{X}]\big|_z = \begin{bmatrix}
    \pE_\mu[1] & \pE_\mu[x_{i_1}] & \cdots & \pE_\mu[X_\phi] & \cdots  \pE_\mu[x_{i_1}x_{i_2}...x_{i_k}]\\
    \pE_\mu[x_{i_1}] & \pE_\mu[x_{i_1}^2] & \cdots &  \pE_\mu[x_{i_1}X_\phi] & \cdots \pE_\mu[x_{i_1}^2x_{i_2}...x_{i_k}]\\
    \vdots & \vdots & \vdots & \ddots & \vdots \\
    \pE_\mu[x_{i_1}x_{i_2}...x_{i_k}] & \pE_\mu[x_{i_1}^2x_{i_2}...x_{i_k}] & \cdots & \pE_\mu[x_{i_1}x_{i_2}...x_{i_k}X_\phi] & \cdots  \pE_\mu[x_{i_1}^2x_{i_2}^2...x_{i_k}^2]
\end{bmatrix}
\]
Even at first glance, if we set $M_{1,t}$ and $M_{2,t}$ to be projection matrices to a subspace of dimension $\hat{r}$ we observe that OptGNN-MC$_r(\textbf{v})$ can simulate projected gradient descent on any $\hat{r}$ less than $r$.  In this sense, OptGNN-MC$_r(\textbf{v})$ can at the very least simulate a dynamic that starts solving the SDP relaxation at $\hat{r} = \sqrt{N}$ and gradually decreases the rank to solve for a fixed point of the greedy dynamic at $\hat{r}=1$ with any schedule of step sizes.  Of course, what it actually learns with backpropagation over a dataset could is a much more diverse set of dynamics that can't be easily described, but can be evaluated as we do in ...          
\NK{Is the discussion around the rank main text worthy? The paragraph on greedy vs SDP relaxations etc is kind of hard to parse. Imo can just assert that this solves the SDP and then elaborate in the supplement}

Unique games curve is given TRUE objective (not relaxed) of value c the best poly time solution.  S(c) is given instances with SDP value c the minimum integral objective.

\section{Lift and Project}
\[
X = \begin{bmatrix}
    x_{00} & x_{01} & \cdots & x_{0N} \\
    x_{10} & x_{11} & \cdots & x_{1N} \\
    \vdots & \vdots & \vdots & \ddots & \vdots \\
    x_{N0} & x_{N1} & \cdots &  x_{NN}
\end{bmatrix}
\]
We begin our discussion of discrete optimization by focusing on quadratic problems subject to quadratic constraints.  Take for example, the vertex cover problem.  

The integer program for vertex cover is as follows

\begin{align*} 
\text{Minimize:} \quad &  \sum_{i \in [N]} x_i\\
\text{Subject to:} \quad & (1-x_i)(1-x_j) = 0 & \forall (i,j) \in E\\
\quad & x_i \in \{0,1\} & \forall i \in [N]
\end{align*}

The global optimum of the integer program is the min vertex cover.  Unfortunately the loss is discrete and not amenable to the tools of continuous optimization. 
Therefore a common approach is to relax the loss to be within a continuous interval. 

\begin{align*} 
\text{Minimize:} \quad &  \sum_{i \in [N]} x_i\\
\text{Subject to:} \quad & (1-x_i)(1-x_j) = 0 & \forall (i,j) \in E\\
\quad & x_i \in [0,1] & \forall i \in [N]
\end{align*}

For sake of symmetry it's helpful to apply a simple affine transform to $x$ so that it's in the interval $[-1,1]$ as so. 

\begin{align*} 
\text{Minimize:} \quad &  \sum_{i \in [N]} \frac{1+x_i}{2}\\
\text{Subject to:} \quad & (1-x_i)(1-x_j) = 0 & \forall (i,j) \in E\\
\quad & x_i \in [-1,1] & \forall i \in [N]
\end{align*}

Although the objective is linear the constraint is quadratic which is the source of the nonconvexity.  The idea of relaxation is to add variables $x_{ij}$ to replace quadratic variables $x_ix_j$ to form a linear program relaxation. 

\begin{align*} 
\text{Minimize:} \quad &  \sum_{i \in [N]} \frac{1+x_i}{2}\\
\text{Subject to:} \quad & 1-x_i-x_j+x_{ij} = 0 & \forall (i,j) \in E\\
\quad & x_i \in [-1,1] & \forall i \in [N]\\
\quad & x_{ij} \in [-1,1] & \forall i,j \in [N]
\end{align*}

The advantage of the above formulation is its convexity, thus making it a convex relaxation.  A popular tightening of the linear program relaxation is the oft studied semidefinite program (SDP) relaxation.  Let $X$ be a symmetric matrix with entries denoting variables defined as follows.
\[
X = \begin{bmatrix}
    \Tilde{x}_{00} & \Tilde{x}_{01} & \cdots & \Tilde{x}_{0N} \\
    \Tilde{x}_{10} & \Tilde{x}_{11} & \cdots & \Tilde{x}_{1N} \\
    \vdots & \vdots & \vdots & \ddots & \vdots \\
    \Tilde{x}_{N0} & \Tilde{x}_{N1} & \cdots &  \Tilde{x}_{NN}
\end{bmatrix}
\]

Replacing the original variables $x_i$ with $\frac{\Tilde{x}_{i0} + \Tilde{x}_{0i}}{2}$ and $x_{ij}$ with $\frac{\Tilde{x}_{ij} + \Tilde{x}_{ji}}{2}$, and adopting the notation of frobenius inner product $\langle \rangle$ we have for adequately defined matrices $C$ and $A_e$ 

\begin{align*} 
\text{Minimize:} \quad &  \langle C,X\rangle\\
\text{Subject to:} \quad & \langle A_{e},X\rangle = 0 & \forall e \in E\\
\quad & X_{ii} = 1 & \forall i \in [N]\\
\quad & X \succeq 0\\
\end{align*}

Although the SDP formulation is convex, owing to the convexity of the spectrahedral cone of psd matrices, it is notoriously more expensive than linear programming.  However, the infamous 'low rank'  overparameterization of the SDP relaxation by Burer and Monteiro is amenable to fast iterative algorithms such as block coordinate descent (message passing).  Noting that   

\begin{align*} 
\text{Minimize:} \quad &  \langle C,VV^T\rangle\\
\text{Subject to:} \quad & \langle A_{e},VV^T\rangle = 0 & \forall e \in E\\
\quad & v_i \in \R^{r} & \forall i \in [N]\\  
\quad &\|v_i\| = 1 & \forall i \in [N]\\
\quad & V = \begin{bmatrix}
    \cdots & v_1 \cdots \\
    \cdots & v_2 \cdots \\
    & \vdots \\
    \cdots & v_N \cdots
\end{bmatrix}\\
\end{align*}

Next we move the linear constraints to the objective by introducing a penalty term $\rho > 0$ 

\begin{align*} 
\text{Minimize:} \quad &  \langle C,VV^T\rangle + \rho\sum_{e \in E}\langle A_{e},VV^T\rangle^2\\
\text{Subject to:}
\quad & v_i \in \R^{r} & \forall i \in [N]\\  
\quad &\|v_i\| = 1 & \forall i \in [N]\\
\quad & V = \begin{bmatrix}
    \cdots & v_1 \cdots \\
    \cdots & v_2 \cdots \\
    & \vdots \\
    \cdots & v_N \cdots
\end{bmatrix}\\
\end{align*}

Now we can design a simple projected gradient descent scheme as follows 

\begin{align*}
\hat{v_i}^{t+1} \defeq v_i^t - \eta \big( 2\sum_{j \in N(i)}C_{ij} v_j + 4\rho \sum_{j \in N(i)} \langle A_{(i,j)},VV^T\rangle A_{(i,j)} V \big)
\end{align*}

\begin{align*}
v_i^{t+1} = \frac{\hat{v}_i^{t+1}}{ \|\hat{v}_i^{t+1}\|}
\end{align*}

Note that the projected gradient descent is a message passing algorithm where neighbors of a node pass a linear form of their messages followed by a nonlinear update that is normalization.  That is to say it's a graph neural network.  

\subsection{Lift and Project Loss}
We refer to the following as the projected loss.  It corresponds to $r=1$ low rank SDP.  Aside from the fact that $x_i \in [-1,1]$, for $\rho$ sufficiently large it is identical to the discrete optimization problem.    
\begin{align*} 
\text{Minimize:} \quad &  \langle C,xx^T\rangle + \rho \sum_{e \in E} \langle A_e,xx^T\rangle^2\\
\text{Subject to:} 
\quad & x_i \in [-1,1] & \forall i \in [N]\\
\end{align*}

Next we define the lifted loss coresponding to the convex relaxation.  

\begin{align*} 
\text{Minimize:} \quad &  \langle C,VV^T\rangle + \rho\sum_{e \in E}\langle A_{e},VV^T\rangle^2\\
\text{Subject to:}
\quad & v_i \in \R^{r} & \forall i \in [N]\\  
\quad &\|v_i\| = 1 & \forall i \in [N]\\
\quad & V = \begin{bmatrix}
    \cdots & v_1 \cdots \\
    \cdots & v_2 \cdots \\
    & \vdots \\
    \cdots & v_N \cdots
\end{bmatrix}\\
\end{align*}

\section{Neural Certification Scheme}
First we define the primal problem 
\begin{align*}
\text{Minimize:} \quad &  \langle C,X\rangle \\
\text{Subject to:} \quad & \langle A_i, X\rangle = b_i & \forall i \in [k]\\
\quad & X \succeq 0
\end{align*}

Next we introduce lagrange multipliers $\lambda \in \mathbb{R}^k$ and $Q \succeq 0$ to form the lagrangian 
\begin{align*}
\mathcal{L}(\lambda,Q,X) = \langle C,X\rangle + \sum_{i \in [k]} \lambda_i (\langle A_i,X\rangle - b_i) - \langle Q,X\rangle
\end{align*}

where 
\begin{multline*}
OPT(X) = \min_{X \succeq 0}\max_{\lambda \in \R,Q \succeq 0}\mathcal{L}(\lambda,Q,X) \\
\geq \min_{V \in \mathbb{R}^{N \times N}}\max_{\lambda}\langle C,VV^T\rangle + \sum_{i \in [k]} \lambda_i (\langle A_i,VV^T\rangle - b_i)\\
\geq \max_{\lambda}\min_{V \in \mathbb{R}^{N \times N}}\langle C,VV^T\rangle + \sum_{i \in [k]} \lambda_i (\langle A_i,VV^T\rangle - b_i)\\
\geq \min_{V \in \mathbb{R}^{N \times N}}\langle C,VV^T\rangle + \sum_{i \in [k]} \lambda^*_i (\langle A_i,VV^T\rangle - b_i) 
\end{multline*}
Where in the first inequality we replaced $X \succeq 0$ with $VV^T$ which is a lower bound as every psd matrix admits a cholesky decomposition.  In the second inequality we flipped the order of min and max, and in the final inequality we chose a specific set of dual variables $\lambda^* \in \R^k$ which lower bounds the maximization over dual variables.  The key is to find a good setting for $\lambda^*$.  

Let 
\begin{align*}
F_\lambda(X) \defeq  \langle C,X\rangle + \sum_{i \in [k]} \lambda^*_i (\langle A_i,X\rangle - b_i) 
\end{align*}

We have by convexity that 

\begin{align*}
F_\lambda(X) -  F_\lambda(\Tilde{X}) \leq \langle \nabla F_\lambda(X), X - \Tilde{X} \rangle = \langle \nabla F_\lambda(X), X\rangle + \langle - \nabla F_\lambda(X) ,\Tilde{X} \rangle \\
\leq \langle \nabla F_\lambda(X), X\rangle - \lambda_{min}(\nabla F_\lambda(X) )\mathrm{Tr}(\Tilde{X})
\end{align*}
Therefore it suffices to upper bound the two terms above, which except for $\mathrm{Tr}(\Tilde{X})$ is entirely comprised of quantities that can be computed from the output of the lift-network.  Now let 

\begin{align*}
H_\lambda(V) \defeq  \langle C,VV^T\rangle + \sum_{i \in [k]} \lambda^*_i (\langle A_i,VV^T\rangle - b_i) 
\end{align*}

We know 

\begin{align*}
\nabla H_\lambda(V) =  2(C + \sum_{i \in [k]} \lambda^*_i A_i)V = 2 \nabla F_\lambda(X) V
\end{align*}

Let 
\begin{align*}
    R_{\lambda,\rho} (V) \defeq  \langle C,VV^T\rangle + \sum_{i \in [k]} \rho (\langle A_i,VV^T\rangle - b_i)^2 + \sum_{i=1}^N \bar{\lambda}_i(\langle e_ie_i^T, VV^T\rangle - 1)
\end{align*}
denote the penalized lagrangian with quadratic penalties for constraints of the form $\langle A_i,X \rangle = b_i$.  

Taking the gradient we obtain 

\begin{align*}
    \nabla R_{\lambda,\rho} (V) \defeq  2CV + \sum_{i \in [k]} 2\rho (\langle A_i,VV^T\rangle - b_i)A_i V + \sum_{i=1}^N 2\bar{\lambda}_i e_ie_i^TV
\end{align*}

Our rule for setting $\lambda^*_i$ is 
\[\lambda^*_i \defeq  2\rho (\langle A_i,VV^T\rangle - b_i)\] 

our rule for setting 
\[\bar{\lambda}_j \defeq \frac{1}{2}\|e_j^T(C + \sum_{i \in [k]} 2\rho (\langle A_i,VV^T\rangle - b_i)A_i) V \| \]

Writing out everything explicitly we obtain the following matrix for 

\begin{align*}
\nabla F_\lambda(V) =  C + \sum_{i \in [k]}  \rho (\langle A_i,VV^T\rangle - b_i) A_i + \sum_{j \in [N]} \frac{1}{2}\|e_j^T(C + \sum_{i \in [k]} 2\rho (\langle A_i,VV^T\rangle - b_i)A_i) V \| e_ie_i^T  
\end{align*}

Which is entirely computed in terms of $V$.  It's certainly possible to come up with tighter certification schemes which we leave to future work.

\textbf{Intuition: } Near global optimality one step of the augmented method of lagrange multipliers ought to closely approximate the dual variables.  After obtaining a guess for the penalized lagrange multipliers we estimate the lagrange multipliers for the norm constraint by approximating $\nabla R_{\lambda}(V) = 0$.  The alternative would have been to solve the linear system for all the lagrange multipliers at once but this runs into numerical issues and degeneracies explained below.    

\textbf{Note:} The reason for splitting the set of dual variables is because the projection operator onto the unit ball is hard coded into the architecture of the lift network. Satisfying the constraint set via projection is different from the soft quadratic penalties on the remaining constraints and require separate handling.

\textbf{Morris Note: } It is important to understand that if we were to have computed $\Tilde{X}$, with all its constraints satisfied we'd have as many lagrange multipliers as $|E| + |V|$ for vertex cover. Indeed $\nabla R_{\lambda,\rho} = 0$ yields $N^2$ linear equalities.  However, many of them can be degenerate and fail to uniquely identify $\lambda$ leading to terrible numerical issues.  For example in vertex cover if only the first coordinate is nonzero then only $N$ linear constraints are active.  This issue is a problem with the bound $\langle A,X\rangle \leq \|A\| \mathrm{Tr}(X)$.  Observe that we may be able to tighten this bound with $\max_{X\succeq 0  \text{s.t} X_{ii} = 1}\langle A,X\rangle $ which computes the max cut relaxation for $A$.

\subsection{Max Cut Certificate}
\begin{align*}
    \lambda_i = \frac{1}{2}\| \sum_{j \in N(i)} w_{ij}v_j\|    
\end{align*}
\subsection{Vertex Cover Certificate}
\begin{align*}
    \lambda_\phi = \frac{1}{2}\| \frac{1}{2}\sum_{i=1}^N w_iv_i + 2\rho\sum_{(i,j) \in E} (1- \langle v_i + v_j,\phi\rangle + \langle v_i, v_j \rangle)(-v_i - v_j)\|    
\end{align*}

\begin{align*}
    \lambda_i = \frac{1}{2}\| \frac{1}{2}w_j + 2\rho\sum_{j \in N(i)} (1- \langle v_i + v_j,\phi\rangle + \langle v_i, v_j \rangle)(-\phi + v_j)\|    
\end{align*}

 \subsection{Quadratic vs Linear objective for maxclique}

The question remains, does there exist a hypothesis in $\mathcal{H}$ that approximates the distributional loss of the ground truth estimator $h^*$ which belongs to a much bigger (infinite) class of hypotheses $\mathcal{H}^*$.  That is we wish to bound 

We adopt the loss minimization convention.  
\begin{align}
\E_{x \in \mathcal{D}}[\hat{h}(x)] - \E_{x \in \mathcal{D}}[h^*(x)] \leq \text{ ? } 
\end{align}

Convex optimizaqiton on a graph is remarkably stable.  Even large perturbations to the inputs do not effect the output substantially.  For intuition, consider convex optimization on a quadratic.  No matter where I initialize my gradient descent, I will converge to the global optimum after a small number of iterations.  If I parameterize the gradient descent as a neural network with infinite layers, I find that the number of samples required to learn convex optimization is far smaller than the number of parameters in the network (infinite).  This is because I know two facts.  Firstly, there is a much smaller network that can represent a near optimal solution (quantified by some parameter $\epsilon$).  Secondly, this network is agnostic to the initialization of the network, and depends solely on the description of the optimization.  In the case of a quadratic this will be some PSD matrix, and in the case of a graph optimization it will be the adjacency matrix of the graph.  Running this idea through the generalization analysis with a carefully constructed set of hypotheses we obtain a weird result.  We can learn with far fewer samples than the number of parameters in the OptGNN.  We apply this intuition to the case of GNN's.  

The hypothesis class $\mathcal{H}^*$ for a $\Phi$ layer OptGNN (way more general than this) is approximated to error $\epsilon$ by the following construction. For any $h \in \mathcal{H}^*$ comprised of matrices $h = \{M_1,M_2,...,M_{\Phi}\}$ .  Let $\textbf{NET}_{\epsilon'}: \R^{d \times d} \rightarrow \R^{d \times d}$ be a function that takes a $d$-by-$d$ matrix $M$ and maps it to an $\epsilon'$ entrywise fine net of $M$.  
That is to say the $(i,j)$'th entry of $\textbf{NET}_{\epsilon'}(M)$ is defined as 
\[\textbf{NET}_{\epsilon'}(M)_{(i,j)} \defeq 
\floor{M_{ij}/\epsilon'}\epsilon'\]

In particular the range of $\textbf{NET}_{\epsilon'}$ has cardinality $[(1/\epsilon')^{d^2}]$.  

We construct an injective map $\Omega: \mathcal{H}^* \rightarrow \mathcal{H}$ as follows  
\begin{align}
\Omega(h) \defeq \Bigg\{
\textbf{NET}_{\epsilon/d^{2L}}\big(M_{\Phi}\big), \textbf{NET}_{\epsilon/d^{2L}}\big(M_{\Phi - 1}\big), \textbf{NET}_{\epsilon/d^{2L}}\big(M_{\Phi - 2}\big), ..., \textbf{NET}_{\epsilon/d^{2L}}\big(M_{\Phi - L}\big)\Bigg\}
\end{align}
Note that the cardinality of the domain of \[\left|\bigcup_{h \in \mathcal{H}^*}\Omega(h) \right| \leq \Big(\frac{d^{2L}}{\epsilon}\Big)^{L}\]
which is independent of $\Phi$ the number of layers of the network.  Furthermore, we know there exists a hypothesis in $\mathcal{H}$ that $\epsilon$ approximates the optimal distributional loss.

\section{Can Neural Networks Learn Gradient Descent?}
In this section we develop some preliminary theoretical explanations for why deep and narrow neural networks can learn to perform difficult optimizations.  Our focus will be on the setting of networks that are truly deep (possibly infinitely deep) and also narrow which is a notoriously difficult setting as most of the study of overparameterized neural networks takes the large width scaling TODO: cite NTK. These networks are overparameterized as they have more parameters than training data.  We formulate a toy model for why such deep networks can generalize.  In particular, as far as the authors are aware, there does not exist an explanation for why an infinite depth network that is narrow can optimize something as simple as a quadratic!  

We adopt a simple toy model aimed to explain why overparameterized networks can learn to minimize quadratic functions.  

Let $\mathcal{D}$ be a distribution over quadratic functions $f_a(x) = a_2x^2 + a_1 x + a_3$.  Here we restrict the domain of $a_1 \in [0,a_{max}]$ so that we're working with convex functions.  We use the notation $\vec{a} = \{a_1,a_2,a_3\}$ such that we draw a dataset comprised of $N$ datapoints  $\vec{a}_1,\vec{a}_2,...,\vec{a}_N \sim \mathcal{D}$.    
Let $\mathbf{\theta} = \{\theta_1,\theta_2,...,\theta_T\} \in [-1,1]$ be a collection of $T$ parameters in a parameter space $\Theta$.  
Let the $\text{LAYER}_{(\theta,\vec{a})}$ function be defined as
\begin{align}
\text{LAYER}_{(\theta,\vec{a})}(x) \defeq x + \theta f'(x) \\
= x_t + \theta_t (2a_2x_t + a_1)
\end{align}
Then for some fixed initial $x_0 \in \R$ we define the $\text{NN}_{(\mathbf{\theta},x_0)}: \R^3 \rightarrow \R$ to be 
\begin{align}
\text{NN}_{(\theta,x_0)}(\vec{a}) = f_{a} \circ \text{LAYER}_{(\theta_T,\vec{a})} \circ \text{LAYER}_{(\theta_{T-1},\vec{a})} \circ ... \circ \text{LAYER}_{(\theta_0,\vec{a})}(x_0) 
\end{align}
To be clear, $x_0$ is not the data.  The data is a distribution over quadratics.  For convenience of notation we will often drop the dependence on $x_0$ and refer to $\text{NN}_{(\theta,x_0)}$ as $\text{NN}_{\theta}$.  
Clearly if every $\theta_i \in \mathbf{\theta}$ is a small negative constants $\eta \leq 1/2a_{max}$ then $\text{NN}_{\mathbf{\theta}}$ would implement some type of gradient descent.  However, for an $T$ layer network it's not at all clear what algorithm $\text{NN}_{\theta}$ would end up implementing.  For $T$ going to infinity, the standard PAC learning perturbation analysis in \lemref{lem:pac-learn} would suggest that $\text{NN}_{\theta}$ would require $T \log(T/\epsilon)$ samples.  This would imply that the $\text{NN}_{\theta}$ would never learn how to minimize a quadratic on datasets of fixed size.  This is dismal!  

To make the discussion more precise, let the empirical loss minimizer $\hat{\theta}$ be defined as follows.  

\begin{align}
\hat{\theta} \defeq \argmin_{\theta \in \Theta} \frac{1}{N}\sum_{i \in [N]}\text{NN}_{\theta}(\vec{a}_i)
\end{align}

Then we have the following result, that even with an infinite number of layers $T$, the neural network still successfully generalizes with a number of samples that is independent of the number of parameters.  In fact the sample complexity is dependent only on the distribution $\mathcal{D}$, the approximation error $\epsilon$, and the failure probability $\delta$.     

\begin{lemma}
For any number of layers $T > \frac{2a_{max}}{\epsilon}$, for any number of samples $N = poly(\epsilon^{-1},\delta^{-1})$ for any distribution $\mathcal{D}$ over quadratics, the empirical loss minimizer $\hat{\theta}$ satisfies  
\[\Pr\left[\left|\frac{1}{N}\sum_{i \in [N]}\text{NN}_{\hat{\theta}}(\vec{a}_i) 
 - \E_{\vec{a}\sim \mathcal{D}}\left[ \min_{x \in [-B,B]} f_{\vec{a}}(x)\right]\right| \geq \epsilon \right] \leq \delta \]
\end{lemma}
           
\begin{proof}

\end{proof}

In conclusion, deep and narrow networks can generalize despite having more parameters than training data.
